# Supplementary material for: Unified description of ground and excited states of finite systems: the self-consistent GW approach
Source: arXiv:1202.3547 source file (2012-09-26)
Supplement: Supplementary file 1 [file supplemental_material.pdf]

# Supporting material: A unified description of ground and excited state properties of finite systems: the self-consistent $GW$ approach

F. Caruso,<sup>1,2</sup> P. Rinke,<sup>1,2</sup> X. Ren,<sup>1,2</sup> M. Scheffler,<sup>1,2</sup> and A. Rubio<sup>1,2,3</sup>

<sup>1</sup>*Fritz-Haber-Institut der Max-Planck-Gesellschaft, Faradayweg 4-6, D-14195 Berlin, Germany*

<sup>2</sup>*European Theoretical Spectroscopy Facility*

<sup>3</sup>*Nano-Bio Spectroscopy group and ETSF Scientific Development Centre, Universidad del País Vasco, CFM CSIC-UPV/EHU-MPC and DIPC, Av. Tolosa 72, E-20018 Donostia, Spain*

In this supplemental material we list the vertical ionization energies (VIEs) of the 30 closed shell molecules shown in Fig. 4, show the sc- $GW$  electron density of the CO dimer and give more details on the implementation of the self-consistent screened Coulomb interaction. Finally, we provide a derivation of the matrix representation of the Galitskii-Migdal formula for the total energy (Eq. 6).

## VERTICAL IONIZATION ENERGIES OF CLOSED-SHELL MOLECULES

Table I reports the quasiparticle HOMO level obtained from  $G_0W_0@HF$ ,  $G_0W_0@PBE$  and sc- $GW$  (present work) and frozen-core sc- $GW$  reproduced from [2]. DFT-LDA eigenvalues are also reported. All ionization energies – with the exception of the sc- $GW$  results reproduced from [2] – were obtained with the FHI-aims code using a Tier 2 numeric atom-centered orbital basis set [3]. The experimental values are taken from the photoemission data compiled in Ref. [1]. A graphical comparison of LDA,  $G_0W_0@HF$ ,  $G_0W_0@PBE$  and sc- $GW$  with experiment is reported in Fig. 4 of the Rapid Communication. The discrepancy between our sc- $GW$  VIEs and those reported in Ref. [2] can probably be traced back to the frozen-core approximation employed in Ref. [2] as we observe larger deviations for molecules composed by heavier atoms (e.g.  $F_2$ ,  $P_2$  and  $SH_2$ ). However, this trend is not observed for the whole set, and a more rigorous study of the effects of the core-valence interaction in sc- $GW$  is therefore needed.

## DENSITY OF CO FROM SC- $GW$

Additional information on the quality of the sc- $GW$  ground state can be obtained from the ground-state density  $n(\mathbf{r})$ . Figure 1 illustrates the effect of many-body correlations in the CO dimer by comparing coupled cluster singles doubles (CCSD) calculations and sc- $GW$  with HF which we obtained using the aug-cc-pVTZ basis set. CCSD and sc- $GW$  both exhibit left-right correlation (density is shifted from the bonding region to the individual atoms) and angular correlation (the angular distribution of charge becomes more pronounced). The similarity between the CCSD and sc- $GW$  density reflects

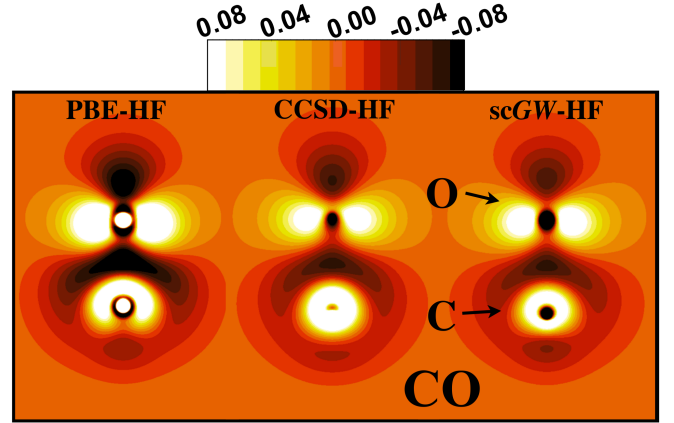

FIG. 1. Difference  $\Delta n(\text{sc-}GW - \text{HF}) = n^{\text{sc}GW} - n^{\text{HF}}$  between the sc- $GW$  and Hartree-Fock densities (right) for the CO dimer, the density differences  $\Delta n(\text{CCSD} - \text{HF})$  (center) and  $\Delta n(\text{PBE} - \text{HF})$  (left) are defined similarly in terms of the CCSD and PBE densities. Dark regions correspond to negative values whereas positive regions are light. Units are  $\text{\AA}^{-3}$  and the calculation was performed using an aug-cc-pVTZ basis set.

the good agreement of the sc- $GW$  dipole moment with the experimental one (see text). In PBE, on the other hand, electron density drifts out of the bond region as a result of the delocalization error, which ultimately leads to an overestimation of the dipole moment (Fig. 1, left).

## COMPUTATION OF THE SCREENED COULOMB INTERACTION

The computation of the polarizability constitutes the main bottleneck of a numerical implementation of the  $GW$  approximation. To avoid the computation of convolutions, the polarizability can be expressed in imaginary time as:

$$\chi_0(\mathbf{r}, \mathbf{r}', \tau) = -iG(\mathbf{r}, \mathbf{r}', \tau)G(\mathbf{r}, \mathbf{r}', -\tau). \quad (1)$$

Here  $i\tau$  labels imaginary time and the Green function is updated at each iteration of the self-consistent loop. Equation 1 is then expanded in an auxiliary basis  $\{P^\mu(\mathbf{r})\}$  by means of the *resolution of the identity* (RI)

TABLE I. Ionization energy for the systems in Fig. 4 evaluated with  $G_0W_0$ @HF,  $G_0W_0$ @PBE, sc- $GW$ . The Hartree-Fock (HF), Kohn-Sham LDA (KS-LDA) and PBE (KS-PBE) eigenvalues are included for comparison. Photoemission experiment are reproduced from [1] and literature sc- $GW$  values are taken from [2].

| Molecule                       | Experiment [1] | $G_0W_0$ @HF | $G_0W_0$ @PBE | sc- $GW$ [2] | sc- $GW$ | HF    | KS-PBE | KS-LDA |
|--------------------------------|----------------|--------------|---------------|--------------|----------|-------|--------|--------|
| C <sub>2</sub> H <sub>2</sub>  | 11.49          | 11.60        | 10.87         | 10.6         | 10.92    | 11.19 | 7.19   | 7.36   |
| C <sub>2</sub> H <sub>4</sub>  | 10.68          | 10.77        | 10.27         | 9.8          | 10.18    | 10.30 | 6.78   | 6.96   |
| CH <sub>3</sub> Cl             | 11.29          | 11.52        | 10.72         | 11.0         | 11.09    | 11.86 | 7.07   | 7.16   |
| CH <sub>4</sub>                | 13.6           | 14.76        | 13.72         | 14.1         | 14.24    | 14.83 | 9.45   | 9.46   |
| Cl <sub>2</sub>                | 11.49          | 11.71        | 10.92         | 10.9         | 11.22    | 12.07 | 7.30   | 7.41   |
| ClF                            | 12.77          | 12.99        | 11.97         | 12.4         | 12.52    | 13.45 | 7.84   | 7.98   |
| CO                             | 14.01          | 14.74        | 13.35         | 13.4         | 13.91    | 15.13 | 9.02   | 9.10   |
| CO <sub>2</sub>                | 13.78          | 14.24        | 13.21         | 13.1         | 13.70    | 10.26 | 5.14   | 5.38   |
| CS                             | 11.33          | 12.96        | 10.69         | 10.8         | 11.26    | 12.58 | 7.34   | 7.39   |
| F <sub>2</sub>                 | 15.7           | 15.98        | 14.44         | 15.2         | 15.93    | 18.23 | 9.45   | 9.64   |
| H <sub>2</sub> CO              | 10.88          | 11.36        | 10.29         | 10.4         | 10.92    | 12.07 | 6.24   | 6.32   |
| H <sub>2</sub> O               | 12.62          | 12.86        | 11.73         | 12.3         | 12.64    | 13.91 | 7.22   | 7.37   |
| H <sub>2</sub> O <sub>2</sub>  | 11.7           | 11.78        | 10.80         | 11.0         | 11.68    | 13.03 | 6.20   | 6.34   |
| HCl                            | 12.74          | 12.77        | 12.11         | 12.2         | 12.36    | 12.98 | 8.04   | 8.14   |
| HCN                            | 13.61          | 13.86        | 13.15         | 12.7         | 13.19    | 13.51 | 9.02   | 9.19   |
| HF                             | 16.12          | 15.99        | 14.98         | 16.0         | 16.22    | 17.76 | 9.64   | 9.81   |
| Li <sub>2</sub>                | 5.11           | 5.31         | 5.26          | 4.6          | 4.92     | 4.92  | 3.21   | 3.22   |
| LiF                            | 11.3           | 11.26        | 10.09         | 11.7         | 11.59    | 13.01 | 6.11   | 6.24   |
| LiH                            | 7.9            | 8.17         | 6.91          | 8.0          | 7.91     | 8.20  | 4.36   | 4.39   |
| N <sub>2</sub>                 | 15.58          | 17.09        | 14.89         | 15.1         | 15.53    | 16.75 | 10.22  | 10.37  |
| Na <sub>2</sub>                | 4.89           | 4.88         | 5.01          | 4.1          | 4.84     | 4.51  | 3.12   | 3.21   |
| NaCl                           | 9.8            | 9.27         | 8.45          | 9.0          | 8.96     | 9.63  | 5.27   | 5.40   |
| NH <sub>3</sub>                | 10.82          | 11.15        | 10.13         | 10.8         | 10.84    | 11.67 | 6.13   | 6.23   |
| P <sub>2</sub>                 | 10.62          | 10.57        | 9.99          | 9.2          | 9.81     | 10.10 | 7.13   | 7.25   |
| PH <sub>3</sub>                | 10.95          | 10.63        | 10.14         | 9.9          | 10.33    | 10.50 | 6.64   | 6.70   |
| SH <sub>2</sub>                | 10.5           | 10.83        | 9.88          | 9.8          | 10.02    | 10.67 | 6.56   | 6.69   |
| Si <sub>2</sub> H <sub>6</sub> | 10.53          | 11.07        | 10.01         | 10.2         | 10.48    | 11.03 | 7.28   | 7.34   |
| SiH <sub>4</sub>               | 12.3           | 13.16        | 12.06         | 12.3         | 12.71    | 13.24 | 8.52   | 8.53   |
| SiO                            | 11.49          | 11.81        | 10.87         | 10.9         | 11.24    | 11.92 | 7.45   | 7.59   |
| SO <sub>2</sub>                | 12.5           | 12.21        | 11.77         | 11.3         | 12.17    | 12.39 | 7.51   | 7.68   |

technique. The auxiliary basis functions  $P^\mu(\mathbf{r})$  are defined to span the Hilbert space generated from the products of numerical atom-centered orbitals  $\{\varphi_i(\mathbf{r})\}$ , so that:

$$\varphi_i(\mathbf{r})\varphi_j(\mathbf{r}) = \sum_{\mu=1}^{N_{\text{aux}}} C_{ij}^\mu P^\mu(\mathbf{r}). \quad (2)$$

$N_{\text{aux}}$  is the total number of auxiliary basis functions, and  $C_{il}^\mu$  are the expansion coefficients. The way to determine  $C_{il}^\mu$  is not unique as different variational procedures may be employed to minimize the error in the expansion in Eq. 2. In the present work, the expansion coefficients  $C_{il}^\mu$  were computed following the RI-SVS approach [4] and we refer to Ref. [5] for a detailed discussion of the technical aspects involved in the computation of the expansion

coefficients. The matrix elements of the polarizability in the auxiliary basis representation are then given by:

$$\chi_0^{\mu\nu}(i\tau) = i \sum_{ijlm} C_{il}^\mu C_{jm}^\nu G_{ij}(i\tau) G_{lm}(-i\tau), \quad (3)$$

where  $G_{ij}$  are matrix element of the Green function in terms of numerical atom centered orbitals (NAO).

Subsequently, the polarizability is Fourier transformed to imaginary frequency, and the screened Coulomb interaction is obtained from

$$W^{\mu\nu}(i\omega) = \sum_{\nu'} V_{\mu\nu'} [1 - V\chi_0(i\omega)]_{\nu'\nu}^{-1}, \quad (4)$$

where  $V_{\mu\nu}$  is the product basis representation of the bare coulomb interaction.

# MATRIX REPRESENTATION OF THE GALITSKII-MIGDAL FORMULA

In atomic units ( $\hbar = e = m = 1$ ), the Galitskii-Migdal formula can be written as [6]:

$$E_{\text{GM}} = -i \int d^3\mathbf{r} dt \lim_{\mathbf{r}' \rightarrow \mathbf{r}} \lim_{t' \rightarrow t^+} \left[ i \frac{\partial}{\partial t} - \frac{\nabla_{\mathbf{r}}^2}{2} + v_{\text{ext}}(\mathbf{r}) \right] G(\mathbf{r}t, \mathbf{r}'t') \quad , \quad (5)$$

where  $v_{\text{ext}}$  is the external (time-independent) potential, and we omitted spin variables. Using the equation of motion for the one-particle Green function:

$$\left[ i \frac{\partial}{\partial t} + \frac{\nabla_{\mathbf{r}}^2}{2} - v_{\text{H}}(\mathbf{r}) - v_{\text{ext}}(\mathbf{r}) \right] G(\mathbf{r}t, \mathbf{r}'t') - \int d\mathbf{r}'' dt'' \Sigma(\mathbf{r}t, \mathbf{r}''t'') G(\mathbf{r}''t'', \mathbf{r}'t') = \delta(\mathbf{r} - \mathbf{r}') \delta(t - t') \quad , \quad (6)$$

where  $v_{\text{H}}$  is the Hartree potential, Eq. 5 may be rewritten in a form more suitable for practical calculations:

$$E_{\text{GM}} = -i \int d^3\mathbf{r} d^3\mathbf{r}'' dt dt'' \lim_{\mathbf{r}' \rightarrow \mathbf{r}} \lim_{t' \rightarrow t^+} [(-\nabla_{\mathbf{r}}^2 + 2v_{\text{ext}}(\mathbf{r}) + v_{\text{H}}(\mathbf{r})) \delta(\mathbf{r} - \mathbf{r}'') \delta(t - t'') + \Sigma(\mathbf{r}t, \mathbf{r}''t'')] G(\mathbf{r}''t'', \mathbf{r}'t') \quad . \quad (7)$$

Making use of the matrix representation of the Green function  $G(\mathbf{r}, \mathbf{r}', \tau) = \sum_{ij} \phi_i(\mathbf{r}) G_{ij}(\tau) \phi_j(\mathbf{r}')$ , the first three terms in Eq. 7 can be rewritten as:

$$\begin{aligned} & -i \int d^3\mathbf{r} dt \lim_{\mathbf{r}' \rightarrow \mathbf{r}} \lim_{t' \rightarrow t^+} [-\nabla_{\mathbf{r}}^2 + 2v_{\text{ext}}(\mathbf{r}) + v_{\text{H}}(\mathbf{r})] G(\mathbf{r}t, \mathbf{r}'t') = \\ & -i \int d^3\mathbf{r} \lim_{\mathbf{r}' \rightarrow \mathbf{r}} [-\nabla_{\mathbf{r}}^2 + 2v_{\text{ext}}(\mathbf{r}) + v_{\text{H}}(\mathbf{r})] \sum_{ij} \phi_i(\mathbf{r}) G_{ij}(\tau = 0^-) \phi_j(\mathbf{r}') = \\ & -i \sum_{ij} G_{ij}(\tau = 0^-) [2t_{ji} + 2v_{ji}^{\text{ext}} + v_{ji}^{\text{H}}] \end{aligned} \quad (8)$$

where we assumed [7] that the Green function depends only on the difference of time variables  $\tau \equiv t - t'$ . We defined, in the last step of Eq. 8 the matrix representation of the kinetic energy operator as  $t_{ij} = \int d^3\mathbf{r} \phi_i(\mathbf{r}) \left[ -\frac{\nabla_{\mathbf{r}}^2}{2} \right] \phi_j(\mathbf{r})$ , and a similar representation for  $v_{ji}^{\text{ext}}$  and  $v_{ji}^{\text{H}}$ . Finally, the last term in Eq. 7 can be rearranged by using the Fourier transform of the Green function and the self-energy  $G(t, t') = \int_{-\infty}^{+\infty} \frac{d\omega}{2\pi} e^{-i\omega(t-t')} G(\omega)$ , and substituting the matrix representation of  $G$ :

$$-i \int d^3\mathbf{r} d^3\mathbf{r}'' dt dt'' \lim_{\mathbf{r}' \rightarrow \mathbf{r}} \lim_{t' \rightarrow t^+} \Sigma(\mathbf{r}t, \mathbf{r}''t'') G(\mathbf{r}''t'', \mathbf{r}'t') = -i \sum_{ij} \int \frac{d\omega}{2\pi} \Sigma_{ji}(\omega) G_{ij}(\omega) e^{i\omega\eta} \quad (9)$$

Summing Eqs. 8 and 9 and separating the self-energy in its exchange and correlation components  $\Sigma_{ij}(\omega) = \Sigma_{ij}^{\text{x}} + \Sigma_{ij}^{\text{c}}(\omega)$ , one can finally rewrite the total electronic energy as:

$$E_{\text{GM}} = -i \sum_{ij} [2t_{ji} + 2v_{ji}^{\text{ext}} + v_{ji}^{\text{H}} + \Sigma_{ji}^{\text{x}}] G_{ij}(\tau = 0^-) - i \sum_{ij} \int \frac{d\omega}{2\pi} \Sigma_{ji}^{\text{c}}(\omega) G_{ij}(\omega) e^{i\omega\eta} \quad (10)$$

We refer to Ref. [8], for a discussion on the evaluation of the Galitskii-Migdal formula directly on the imaginary frequency axis.

[1] <http://cccbdb.nist.gov/>.

[2] C. Rostgaard, K. W. Jacobsen, and K. S. Thygesen, Phys. Rev. B **81**, 085103 (2010).

[3] V. Blum, R. Gehrke, F. Hanke, P. Havu, V. Havu, X. Ren, K. Reuter, and M. Scheffler, Comp. Phys. Comm. **180**, 2175 (2009).

[4] O. Vahtras, J. Almlf, and M. Feyereisen, Chem. Phys. Lett. **213**, 514 (1993).

[5] X. Ren, P. Rinke, V. Blum, J. Wieferink, A. Tkatchenko, A. Sanfilippo, K. Reuter, and M. Scheffler, New J. of Phys. **14**, 053020 (2012).

[6] A. L. Fetter and J. D. Walecka, *Quantum Theory of Many-Particle Systems* (Dover Publications, 2003).

[7] This assumption is fully justified for systems described by a time-independent Hamiltonian.

- [8] P. García-González and R. W. Godby, Phys. Rev. B **63**, 075112 (2001).
